# Supplementary material for: Fair, Manipulation-Robust, and Transparent Sortition
Source: arXiv:2406.15009 source file (2024-06-26)
Supplement: Supplementary file 1 [file appendix-pointer.tex]

\newpage
\section{Appendix}
All supplemental materials for this paper can be found at the following permanent link: [link].
